# Supplementary material for: Topological analysis reveals multiple pathways in molecular dynamics
Source: arXiv:2412.20580 ancillary file (2025-01-05)
Supplement: Supplementary file 1 [file supporting_information.pdf]

Supporting Information for:

# Topological analysis reveals multiple pathways in molecular dynamics

Luca Donati,[1,2] Surahit Chewle,[2] Dominik St. Pierre,[3,2] Vijay Natarajan,[4,2] and Marcus Weber[2]

[1)]*Freie Universität Berlin, Department of Mathematics and Computer Science, Arnimallee 22, D-14195 Berlin*

[2)]*Zuse Institute Berlin, Takustr. 7, D-14195 Berlin, Germany*

[3)]*Freie Universität Berlin, Department of Biology, Chemistry and Pharmacy, Arnimallee 22, D-14195 Berlin*

[4)]*Indian Institute of Science, Bangalore, India*

(*Electronic mail: donati@zib.de)

## I. Additional description of ISOKANN algorithm and related figures

Figs. S1, S2, S3, S4 show the $\chi$-function (A), the loss functions (B) and the $\chi$-convergence (C), respectively for the two-dimensional system, the 33-Dichloroisobutene molecule, the VGVAPG hexapeptide and the villin headpiece subdomain.

The $\chi$-function was determined by means of the ISOKANN algorithm that iteratively trains a Feedforward Neural Networks (FNNs). The training of the FNN takes place via a nested loop:

- The outer for-loop is the actual modified power method that converges the arbitrary function $f_k$ to the $\chi$-function:

$$\begin{cases} f_{k+1} = S\mathscr{K}_\tau f_k \\ \lim_{k\to\infty} f_{k+1}(x_{0,n}) = \chi . \end{cases} , \tag{S1}$$

  where $S$ is the shift-scale function $S$ as in eq. 16 and $\mathscr{K}_\tau$ is the Koopman operator. We call "iterations" the number of times this loop is applied. In order to verify convergence, we solve the linear regression problem

$$\min_{a_1,a_2} \|f_{k+1} - a_1 f_k - a_2\| , \tag{S2}$$

  and verify that the slope $a_1$ is

$$1 - \varepsilon < a_1 < 1 + \varepsilon , \tag{S3}$$

  where $\varepsilon$ is a small threshold. Figs. S1-(C), S2-(C), S3-(C), S4-(C) show the value $a_1$ at each iteration.

- The internal for-loop is the training of the FNN that takes place at each iteration $k$ using techniques like batch processing, early stopping and $L^2$-regularization to ensure robust performance and to prevent over-fitting. The training loss function is the Mean Squared Error (MSE) between the model's predictions and the actual target values:

$$MSE = \frac{1}{N}\sum_{i=1}^{N}(f_{k_i} - \hat{f}_{ki}) , \tag{S4}$$

  where $f_{k_i}$ are the true values of the function $f_k$ evaluated at iteration $k$, $\hat{f}_{ki}$ are the corresponding predictions, and $N$ is the number of samples. Before FNN training begins, the

initial dataset, i.e. the dataset of states $X_0$ representing the state space, is divided into training states (80%) and test states (20%) which are used to estimate the validation loss:

$$MSE^{\text{val}} = \frac{1}{N} \sum_{i=1}^{N} (f_{k_i}^{\text{val}} - f_{k_i}) \,, \tag{S5}$$

We call "epochs" the number of times this loop is applied.

The Python code of the ISOKANN implementation used is available at `https://github.com/donatiluca/MoKiTo`.

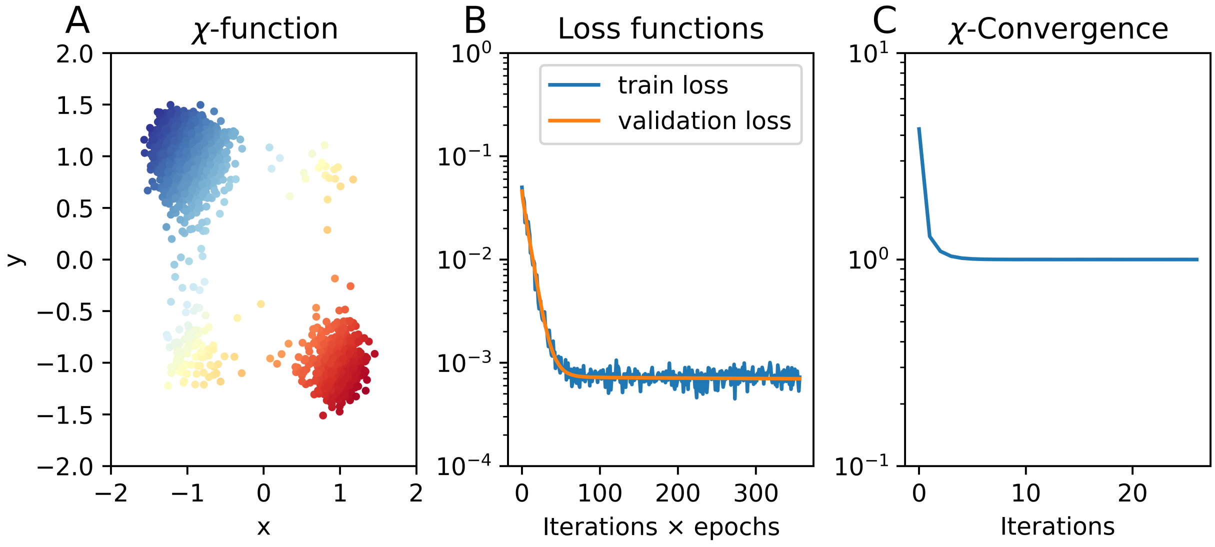


FIG. S1. (A) $\chi$-function of the two-dimensional system projected onto the Cartesian coordinates $x$ and $y$; (B) Validation and training loss functions; (C) $\chi$-convergence.

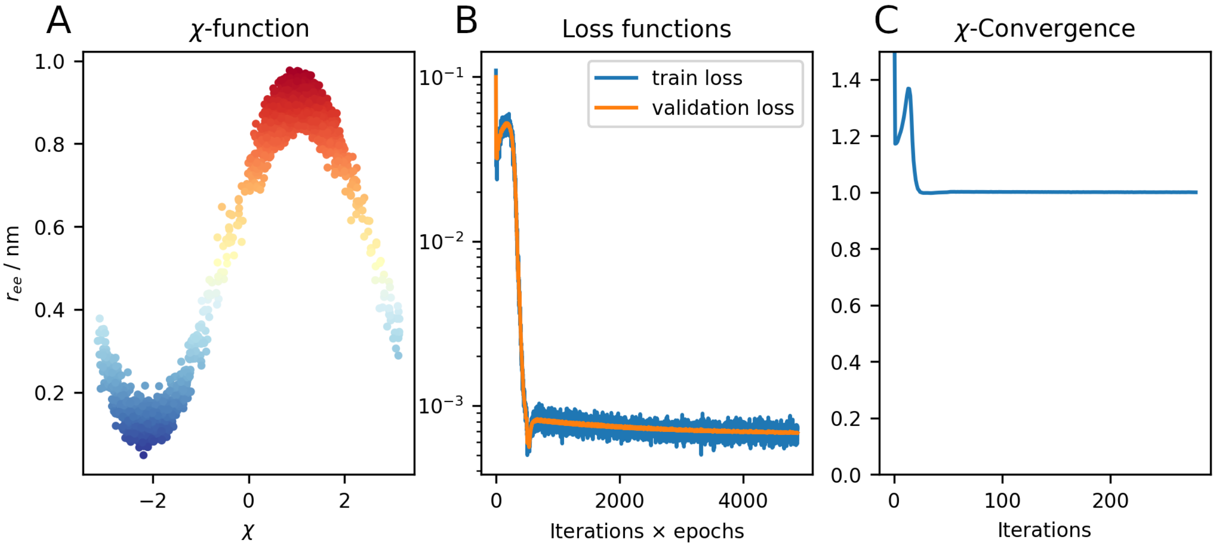


FIG. S2. (A) $\chi$-function of 33-Dichloroisobutene molecule projected onto the torsion angle $\Psi$; (B) Validation and training loss functions; (C) $\chi$-convergence.

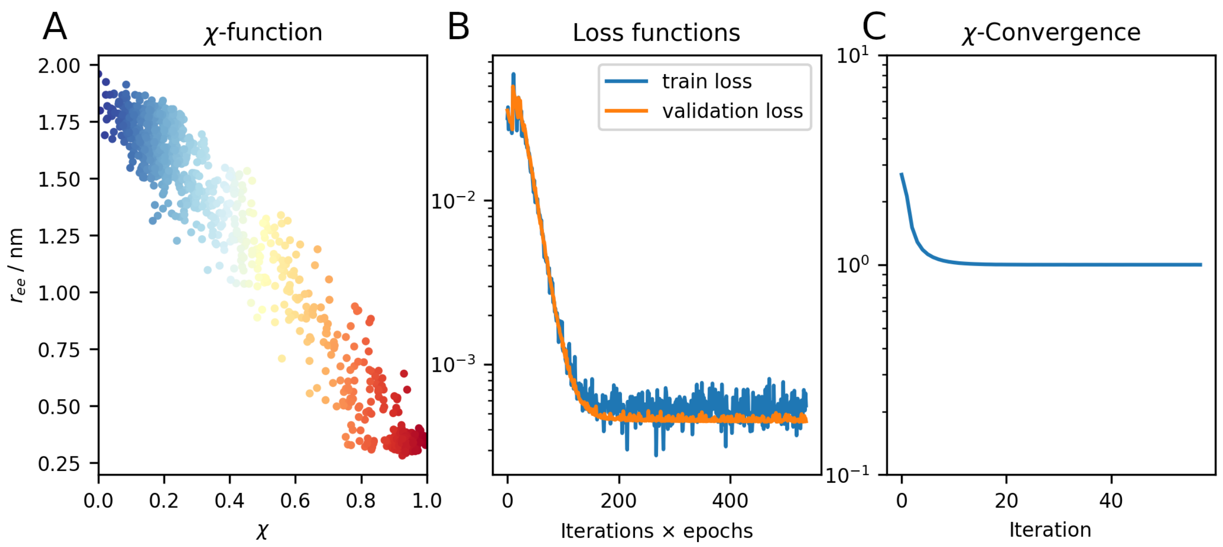


FIG. S3. (A) $\chi$-function of hexapeptide VGVAPG projected onto the end-to-end distance $r_{rr}$; (B) Validation and training loss functions; (C) $\chi$-convergence.

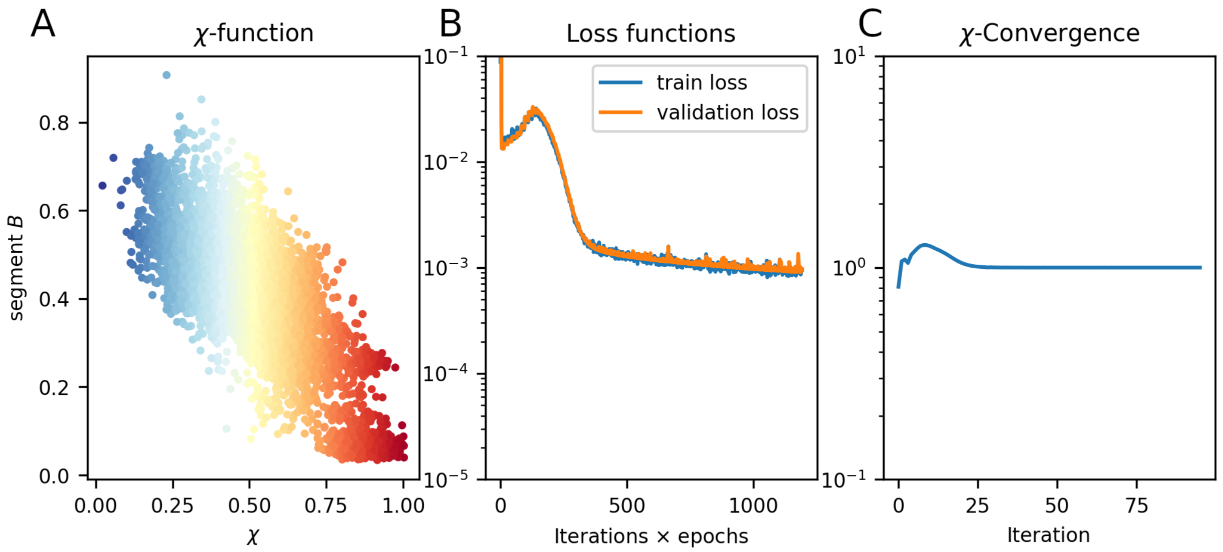


FIG. S4. (A) $\chi$-function of villin projected onto the RMSD of the segment $B$; (B) Validation and training loss functions; (C) $\chi$-convergence.
